# Supplementary material for: Self-supervised surface-related multiple suppression with multidimensional convolution
Source: arXiv:2505.00419 source file (2025-05-01)
Supplement: Supplementary file 1 [file Appendix.tex]

\section{\textsc{SUPPLEMENTARY INFORMATION}}
% \vspace{8pt} \\ 
Supporting information for section X
